# Supplementary material for: How generic is eternal inflation?
Source: arXiv:2111.14218 source file (2021-12-26)
Supplement: Supplementary file 1 [file app_perturbations.tex]

% The action for the unperturbed field $\phi$ and the metric $g_{\mu\nu}$ is given by
% \begin{equation} S = \int \dx^4 x\, \sqrt{-g} \left[ -\frac12 g^{\mu\nu} \partial_\mu \phi \partial_\nu \phi - V(\phi) \right] + \frac{M_P^2}{2} \int \dx^4 x \, \sqrt{-g} \, R \label{action_general} \end{equation}
Let us adopt the ADM parameterization for a general line element
\[ g_{\mu\nu} \dx x^\mu \dx x^\nu =  -N^2 \dx t^2 + h_{ij} (\dx x^i + N^i \dx t) (\dx x^j + N^j \dx t) \]
where $N$ and $N^i$ are the lapse and shift functions, respectively, and $h_{ij}$ is the metric of 3-space.  The scaling of the volume element is then $ \sqrt{-\abs{g_{\mu\nu}}} = \sqrt{h}N $, with $h \equiv \det h_{ij}$.
We further define the quantity
$ E_{ij} \equiv \dot h_{ij} - N_{[i;j]} $ and $E \equiv h^{ij} E_{ij} $.
The action for the scalar field $\phi$ in a background spacetime described by $g_{\mu\nu}$ may then be expressed
% in terms of which the scalar curvature takes the form
% \[ R = 
\[ S = \int \dx t \, \dx^3 x \, \sqrt{h} N \left[ \frac{(\partial_0 \phi - h^{ij} N_i \partial_j \phi)^2}{2 N^2} - \frac12 h^{ij} \partial_i \phi \partial_j \phi - V(\phi) + \frac{M_P^2}{2 N^2} (E_{ij} E^{ij} - E^2) \right] \]
Varying the action with respect to the lapse and shift functions, we obtain
\begin{align*}
% \fdx{S}{N} &= - \frac{(\partial_0 \phi - N^i \partial_i \phi)^2}{2 N^2} - \frac12 h^{ij} \partial_i \phi \, \partial_j \phi - V(\phi) - \frac{M_P^2}{2 N^2} (E_{ij} E^{ij} - E^2) \\
 \fdx{S}{N^i} &= - \frac{(\partial_0 \phi - 2 N^j \partial_j \phi)}{2 N} \, \partial_i \phi + \left[ \frac{M_P^2}{N} \delta^{jk} (E_{ik} - E \delta_{ik}) \right]_{;j} 
 \end{align*}
In the Hamiltonian formalism, the lapse and shift functions are Lagrange multipliers enforcing the Hamiltonian and momentum constraints, so we take the variation with respect to $N^i$ to vanish uniquely, rather than only in a classical limit.
Restricting the metric to FLRW spacetime with flat spatial hypersurfaces, we have 
\[ h_{ij} = a^2(t) \delta_{ij},\quad N = 1+\alpha,\quad N^i = \beta^i,\quad\text{and}\;\; E_{ij} \to a \dot a \delta_{ij} = a^2 H \delta_{ij} \]  
where $\alpha$ and $\beta^i$ are taken to be small.
Furthermore, we introduce perturbations to the scalar field $\phi(t,\vec x) \to \phi_0(t) + \delta \phi(t,\vec x)$, with $\phi_0(t)$ being the homogeneous expectation value that evolves classically.
We can treat $\phi_0$ as a classical field and $\delta\phi$ as the only new quantum field.
Up to lowest order in $\delta\phi$, $\delta S/\delta N^i \equiv 0$ becomes
\begin{align*}
\dot\phi \, \partial_i \delta\phi - 2N^j \partial_j \delta\phi \, \partial_i \delta\phi \approx \dot\phi \, \partial_i \delta\phi &= M_P^2 N \left[ \frac{1}{N} \delta^{jk} (a \dot a - 3 a \dot a) \delta_{ik} \right]_{;j} = 2 M_P^2 a^2 H \partial_i \alpha
% \\
%  \frac{\dot\phi}{1+\alpha} \partial_i \delta\phi &= M_P^2 \left[ \frac{-\partial_j \alpha}{1+\alpha} (-2 a^2 H) \delta_{i}^j \right] 
\end{align*}
Since only $\delta\phi$ and $\alpha$ vary in space, from this we can assume
$ \delta\phi = {2 M_P^2 a^2 H} \, \alpha/\dot\phi $.
% On the RHS, only $\alpha$ varies in space, so we have
% \[ \dot\phi \, \partial_i \delta\phi = 2 M_P^2 a^2 H \partial_i \alpha \]
\[ S = \int \dx t \, \dx^3 x \, a^3 \left[ \frac{(\dot\phi + \dot{\delta\phi} - \beta^i \partial_i \delta\phi )^2}{2 (1+\alpha)^2} - \frac{1}{2a^2} \partial^i \delta\phi \partial_i \delta\phi - V(\phi) - V'(\phi) \delta\phi - \frac12 V''(\phi) \delta\phi^2 \right] \]
We aim to expand around the classical solutions $\phi(t)$ with $N^i \approx 0$ and $N \approx 1$, so we keep only terms that do not appear in the action for the classical solution and are up to quadratic in small quantities $\delta\phi$, $\alpha$, $\beta^i$.
\[ \delta S = \int \dx^4 x \, a^3 \left[ \frac{\dot{\delta\phi}^2}{2} + (1- 2\alpha) \dot\phi \dot{\delta\phi} - \frac{1}{2 a^2} \partial^i \delta\phi \partial_i \delta\phi - \frac12 V''(\phi) \delta\phi^2 \right] \]
\[ \dot\phi \, \dot{\delta\phi} = \dot\phi \ddx{}{t} \left( \frac{2 M_P^2 \alpha H}{\dot\phi a^2} \right) \]
So the $2\alpha \dot\phi\dot{\delta\phi}$ term is quadratic in the small parameter $\alpha$.  Using integration by parts and keeping only terms up to second order in the field perturbation $\delta\phi$, we have
\[ S_{(2)} = \int \dx^4 x \, \frac{a^3}{2} \left[ \dot{\delta\phi}^2 - \frac1{2a^2} \partial^i \delta\phi \partial_i \delta \phi - \mathcal M^2 \delta\phi^2 \right] \]
where
\[ \mathcal M^2 = V''(\phi) - \frac1{a^3 M_{\text{P}}^2} \ddx{}{t} \left( \frac{a^3}{H} \dot\phi^2 \right) \]
% \[ \mathcal M^2 = \ddx{}{t} \ddx{(-3 H \dot\phi)}{\dot\phi} - \frac1{a^3} \ddx{}{t} \left( \frac{a^3}{H} \dot\phi^2 \right) \]
Recall that $V'(\phi) \approx -3 H \dot\phi$ in the slow roll approximation, implying that $V''(\phi) \approx -3 \dot H \approx 0$.
Adopting the conformal time coordinate $ \dx\tau = a(t)^{-1} \dx t $ and making the variable substitutions
$v \equiv a \,\delta \phi $, $z \equiv a \phi' / H$, where a prime denotes a derivative with respect to conformal time
\[ S_v = \frac12 \int \dx\tau \, \dx^3 x \, \left[ (v'')^2 + \partial^i v \partial_i v + \frac{z''}{z} v^2 \right] \]
