# Supplementary material for: How generic is eternal inflation?
Source: arXiv:2111.14218 source file (2021-12-26)
Supplement: Supplementary file 2 [file app_prefactor.tex]

\subsubsection{Prefactor Calculation in the Thin-Wall Approximation }

\paragraph{ Coordinate Systems }
This is based on the nucleation rates paper by Garriga \cite{Garriga1994}.

% First let us define coordinates on the de Sitter space embedded in 5-D Minkowski space.  
Let $X^A$, $A \in \{0,1,2,3,4\}$ locate points on the de Sitter hyperboloid in the coordinates of the embedding space.
% In terms of the flat slicing coordinates in de Sitter space $x^\mu$, they are
% \begin{align*}
% X^0 &= H^{-1} \sinh Ht + \tfrac12 H \vec x^2 e^{Ht} \\
% X^d &= H^{-1} \cosh Ht - \tfrac12 H \vec x^2 e^{Ht} \\
% X^J &= x^J e^{Ht}, \; J \in \{ 1, \dots, N \} \end{align*}
Upon Wick rotation of the time coordinate, $3{+}1$ deSitter space becomes a 4-sphere of radius ${H^{-1}}$ embedded in 5-D Euclidean space. 
\[ (X_E^0)^2 + \sum_{J=1}^d (X^J)^2 = H^{-2}, \quad\text{where}\quad X_E^0 = i X^0 \]
Let us define the coordinate system so that the bubble is centered at the point where the $X^d$ axis intersects the 4-sphere.
Let $\Sigma$ denote the 3-D history of the bubble wall.  (If we supress 2 dimensions to represent the Euclidean de Sitter space as a 2-sphere embedded in 3-space, then $\Sigma$ is a circle of radius $R_0$ inscribed on that sphere around the $+X^d$ axis.)  Let $\xi^a$ denote the coordinates within $\Sigma$, with $a \in \{1,2,3\}$.  Let $\hat n(\xi^a)$ denote the unit vector at a point on $\Sigma$ pointed in the unique direction orthogonal to $\Sigma$ within the 4-sphere.  
\[ \hat n(\xi^a) \perp \Sigma(\xi^a) \]
In the coordinates of the embedding space, the components of $\hat n$ are
\[ \hat n = n^A e_A, \; n^A = H R_0^{-1} (\vec x(\xi^a) \omega_0,\, - R_0^2) \]
where $\vec x$ is the displacement to the point on $\Sigma$ from the center of the 4-sphere in the embedding space.
Here $\omega_0$ is
\[ \omega_0 = H^{-1} \cos \theta_0 \]
and $\theta_0$ is the angle between the $+X^d$ axis and a ray eminating from the center of the 4-sphere in the embedding space and passing through a point on $\Sigma$.

The calculation of the transition amplitude above accounts for only the largest contributions from the classical Euclidean trajectory.  In order to compute the full transition rate, we must account for perturbations to that trajectory that add next to leading order contributions to the transition rate.  This adds a {\it pre-factor} to the original
$ \Gamma = A e^{-S_{\text{E}}} $.
We can consider these to be perturbations to the shape of the bobble in the 5D Euclidean embedding space.

Let us parameterize small perturbations of the shape of $\Sigma$ in terms of a scalar field $\phi(\xi^a)$, with support on $\Sigma$.  If $\phi(\xi^a)$ is positive, then the perturbed surface $\Sigma'$ sticks out of the original $\Sigma$ in the vacinity of $\xi^a$, while a negative value means $\Sigma'$ lies inside $\Sigma$ at that point.  The displacement of the surface in terms of coordinates defined on the 4-sphere is
\[ \delta x^\mu = \sigma^{-1/2} \phi(\xi^a) n^\mu \]
Here $\sigma$ could be any mass scale, and we have chosen the energy per unit surface area (the bubble tension) to simplify things.

The equation of motion for the scalar field $\phi$ must take the form
\[ - \Delta \phi + M^2 \phi = 0 \]
for some constant $M$, whose value can be deduced from symmetry arguments below.

% \paragraph{Zero Modes and Normalization}
An $O(5)$ rotation of the Euclidean embedding space amounts to only a translation of the bubble in de Sitter space.  
Since $\phi$ was introduced to parameterize perturbations in the {\it shape} of the bubble wall, we don't want to include these \emph{zero modes} in the calculation of the transition probabilities. Those probabilities are governed by the Euclidean action, into which $\phi$ first enters at second order
\[ S_{\text{E}}^{(2)}[\phi] = - \frac12 \int d^3\xi \, \sqrt{-\gamma} \, \phi (\Delta - M^2) \phi \]
so we must ensure that solutions $\phi_0(\xi^a)$ corresponding to these modes result in $S_{\text{E}}^{(2)}[\phi] = 0$.

% Rotating by $\alpha$ in the $X^J{-}X^d$ plane, we have
% \[ \delta X^J = \alpha X^d \qquad \delta X^d = - \alpha X^J \]
% The magnitude of the displacement of $\Sigma$ induced by this infinitesimal rotation is
% \[ M^{-1/2} \phi (\xi^a) = n^A \delta X_A(\xi^a) = \alpha (H R_0)^{-1} X^J(\xi^a) \]
Consider taking two spherical shells that completely overlap, and then infinitesimally separating them along one axis.  (This is the infinitesimal form of the rotation described above.) In one hemisphere, the displacement is entirely positive, while it is entirely negative on the other hemisphere, with a zero crossing at the great circle dividing the two.  Since the scalar field has support on the surface of a sphere, we can expand it in terms of spherical harmonics.  In this expansion, only the harmonics with $L = 1$ will contribute, since any other value of $L$ gives the wrong number of zero crossings.  The expansion then takes the form
\[ \phi_0(\xi^a) = \sum_{J} C_{1J} \phi_{1J}(\xi^a) \]
where $\phi_{LJ}(\xi^a)$ are the spherical harmonics with appropriate normalization.  (The index $J$ stands for what could be expessed as $N-1$ different indices ${m_1,\dots,m_{n-1}$ corresponding to the ``azimuthal'' angles on the higher dimensional sphere; $L$ is separated out because it alone determines the eigenvalue.)
The eigenvalue of $\Delta$ for these harmonics gives us $M^2$:
% \[ \Delta \phi_0 = \lambda_1 \phi_0 \]
\[ \lambda_L = -R_0^2 L(L + 2) = -3 R_0^2 \quad \text{for} \; L=1 \]
% \[ \therefore \Delta \phi + 3 R_0^2 \phi = 0 \]
% \[ X^J \in \{ \text{spherical harmonics L = 1} \}:  \]%
So we must have $M^2 = -3R_0^2$.  
% To satisfy orthonormality conditions, the normalization must be
% \[ \phi_{1J}(\xi) = \left( \frac{4}{R_0^2 S_3(R_0)} \right)^{1/2} X^J(\xi)  \implies
% \int \dx \xi^3 \, \sqrt{-\gamma} \, \phi_{1I} \phi_{1J} = \delta_{IJ} \]
For our above definition of $\phi_0(\xi)$ in terms of the $\phi_{1J}$ to hold, the harmonic coefficients for an infinitesimal transformation of this type must take the form
\[ \dx C_{1J} = H^{-1} \dx \alpha_J \left( \frac{\sigma S_3(R_0)}{4} \right)^{1/2} \]

% \paragraph{Abusing Quantum Theory}
The quantum partition function for a thin-walled bubble, with N-D surface $\Sigma$ corresponding to its Wick-rotated world sheet, is
% \[ Z = \int D\Sigma(x^A)\, e^{-S_{\text{E}}[\Sigma]} \]
where the integral is over surfaces $\Sigma(x^A)$, up to a translation in de Sitter space.  We can approximate the partition function by only considering paths that resemble multi-instanton solutions.  Expanding the action around the instanton solution $\bar\Sigma$, we have
% \[ Z_k = e^{-k \bar S_{\text{E}}} \]
% \[ S_{\text{E}}[\Sigma] \approx S_{\text{E}}[\bar\Sigma] + \frac12 \int \dx\xi_1 \dx\xi_2 \left. \fdx{^2S_{\text{E}}}{\phi(\xi_1) \delta\phi(\xi_2)} \right\rvert_{\phi = 0} \delta\phi(\xi_1) \delta\phi(\xi_2) = \bar S_{\text{E}} + S_{\text{E}}^{(2)}[\phi(\xi^a)] \]
% The partition function then approximates to
\[ Z  = \int D\Sigma(x^A)\, e^{-S_{\text{E}}[\Sigma]} \approx \sum_{k=0}^\infty \frac{e^{-k \bar S_{\text{E}}}}{k!} \left( \int D \phi \, e^{-S_{\text{E}}^{(2)}[\phi]} \right)^k = \exp {Z_1} \]
where $Z_1$ is the contribution from a single instanton.
% \[ Z_1 \equiv e^{-\bar S_{\text{E}}} \int D \phi \, e^{-S_{\text{E}}^{(2)}[\phi]} \]
% \[ S_{\text{E}}^{(2)}[\phi] = - \frac12 \int d^3\xi \, \sqrt{-\gamma} \, \phi (\Delta - M^2) \phi \]
%
And the functional integral is parameterized in terms of the coefficients $C_{LJ}$.
% \[ D \phi = \prod_{LJ} \mu \frac{\dx C_{LJ}}{(2\pi)^{1/2}} \]
Expanding $\phi$ in terms of $\phi_{LJ}$ and taking advantage of orthonormality, we have
\[ Z_1 \equiv e^{-\bar S_{\text{E}}} \int \prod_{LJ} \mu \frac{\dx C_{LJ}}{(2\pi)^{1/2}} \, \exp \left( -\frac12 \sum_{LJ} \frac{(\mu C_{LJ})^2}{\mu^2 (M^2 - \lambda_L)^{-1}} \right) \]
(We ignore the fact that changing $\phi$ affects the geometry of the bubble, and therefore the form of the 3-metric $\gamma_{ij}$.) This now takes the form of a Gaussian integral, and can be re-expressed as the determinant of an operator (the inverse covariance matrix)
\[ Z_1 = e^{-\bar S_{\text{E}}} \left( \det \left[ (\mu R_0)^{-2} \hat O \right] \right)^{-1/2} \]
where $ \hat O \equiv R_0^2 ( -\Delta + M^2 ) $ with eigenvalues \[ \Lambda_L = R_0^2 (-\lambda_L + M^2) = R_0^2 (\lambda_1 - \lambda_L) \]
The parameter $\mu$ has dimensions of mass, so both $\mu R_0$ and the operator $\hat O$ are dimensionless.  Evaluating the determinant using magic, we have
\[ \det \left[ (\mu R_0)^{-2} \hat O \right] = (\mu R_0)^{-2 \zeta(0)} e^{-\zeta'(0)} \]
where $\zeta(z)$ is a generalized zeta function customized for $\hat O$, and $\zeta'(z) \equiv \dx \zeta/\dx z$
\[ \zeta(z) \equiv \zeta_{\hat O} (z) = \sum_L g_L \Lambda_L^{-z} \]
where $g_L = (L+1)^2$ is the degeneracy of spherical harmonics with a given $L$.
% \[ g_L = (L+1)^2 \]
% \[ g_L = \frac{(2L + N - 1)(N+L-2)!}{L! \, (N-1)!} = \frac{ (L+1) (L+1)! }{L!} \]

\paragraph{Flat Space Limit}
If we denote the chemical potential -- a (fictitious) free energy associated with just adding a bubble to our Euclidean block universe -- as $\tilde\mu$, then the partition is modified as
\[ Z \approx \sum_{k=0}^\infty \frac{e^{-k (\bar S_{\text{E}} - \tilde\mu \beta)}}{k!} \left( \int D \phi \, e^{-S_{\text{E}}^{(2)}[\phi]} \right)^k = \exp {\left(e^{\tilde\mu\beta} Z_1\right)} \]
where $\beta$ is the thermodynamic $\beta$ associated with temperature of the de Sitter space, which depends on $H$.  We then express the equilibrium number of bubbles in terms of the partition function as
\[ \mathcal N = \left. \frac1{\beta Z} \pdx{Z}{\tilde\mu} \right\rvert_{\beta,V} = e^{\tilde\mu \beta} Z_1 \]
% gives us the expectation value for the number of bubbles produced.  
Since no strictly per-bubble energy cost is actually incurred, we may set $\tilde\mu$ to zero, and obtain
% \[ \dx \mathcal N = \dx Z_1 = \left( \frac{\sigma S_N(R_0)}{2\pi \left(\frac{N+1}{2}\right)} \right)^{\frac{N+1}{2}} \abs{ {\det}' \left[ (\mu R_0)^{-2} \hat O \right]} ^{-1/2} e^{-\bar S_{\text{E}}} \, \dx t \, \dx V \]
\[ \dx \mathcal N = \dx Z_1 = \left( \frac{\sigma S_3(R_0)}{4\pi} \right)^{2} \abs{ {\det}' \left[ (\mu R_0)^{-2} \hat O \right]} ^{-1/2} e^{-\bar S_{\text{E}}} \, \dx t \, \dx V \]
The first factor is the Jacobian associated with converting from spherical harmonic coefficients $C_{LJ}$ of the wall perturbation field $\phi$ to Minkowski coordinates as the variables of integration.  The second factor is the closed form result of the Gaussian integral giving quantum corrections to second order in $\phi$.  (The prime indicates that the zero eigenvalues for the $L=1$ coefficients are excluded from the determinant, allowing it to evaluate to a nonzero value.)  These two terms make up the prefactor.

For bubble nucleation in $3{+}1$ dimensions, $\zeta(0) = 0$, and we can express $\zeta'(z)$ in terms of the derivative of the Riemann zeta function $\zeta_R(z)$ and constants (again using magic).
\[ \ddx{\mathcal N}{t \, \dx V} = \frac{\Gamma}{V} = \left( \frac{\sigma S_3(R_0)}{8\pi} \right)^2 \frac{4 R_0^{-4}}{\pi^2} \, e^{\zeta'_{R}(-2)} e^{-\bar S_{\text{E}}} \]
Substituting $S_3(R_0) = 2\pi^2 R_0^3$ and $e^{\zeta_R'(-2)} = 0.9700$, this becomes
\[ \ddx{\mathcal N}{t \, \dx V} = \frac{\Gamma}{V} = \left( \frac{\sigma \pi R_0^3}{4} \right)^2 \frac{4 R_0^{-4}}{\pi^2} \times 0.97 \times e^{-\bar S_{\text{E}}} \]
\[ \ddx{\mathcal N}{t \, \dx V} = \frac{\Gamma}{V} = 0.243 \times (\sigma R_0)^{2} \, e^{-\bar S_{\text{E}}} \]
% \[ \ddx{\mathcal N}{t \, \dx V} = \frac{\Gamma}{V} = 0.243 \times \frac{9 \sigma^4}{9 H^2 \sigma^2 + \Delta V^2} \, e^{-\bar S_{\text{E}}} \]
% \[ \ddx{\mathcal N}{t \, \dx V} = \frac{\Gamma}{V} = 0.243 \times \left( H^{-2} \sigma^2 \sin^2 \Omega \, \right) e^{-\bar S_{\text{E}}} \]

\paragraph{de Sitter Space}

\[ \dx \mathcal N = \left( {\det}' \left[ (\mu R_0)^{-2} \hat O \right] \right)^{-1/2} e^{-\bar S_{\text{E}}} \prod_{J=0}^{d-1} (2\pi)^{-1/2} \dx C_{1J} \]
If infinitesimal translations of the bubble in de Sitter space correspond to $L=1$ spherical harmonic contributions to $\phi$, then only those coefficients need be included in this integral over spacetime.
\[ \lambda = \left.\frac{\Gamma}{V}\right\rvert_{\text{flat}} = \left( \frac{\sigma S_N(R_0)}{2\pi(N+1)} \right)^{\frac{N+1}2} \left( {\det}' \left[ (\mu R_0)^{-2} \hat O \right] \right)^{-1/2} e^{-\bar S_{\text{E}}} \]
We first express $\dx Z_1$ in terms of the rotation angles of the infinitesimal rotations that generate zero modes.  (The Jacobian factor in $\lambda$ helps us smoothly change variables.)
\begin{align*}
% \dx \mathcal N &= \lambda H^{-4} \prod_{J=0}^3 \dx \alpha_J \\
% \intertext{We can think of the product of angles as a 4-D solid angle on the 4-sphere of radius $H^{-1}$.}
\dx \mathcal N & = \lambda H^{-4} \prod_{J=0}^3 \dx \alpha_J = \lambda H^{-4} \, \dx \Omega \\
\intertext{The quantity $H^{-4}\dx\Omega$ is the infinitesimal contribution to the surface area of the 4-sphere.  Rotating back to Lorenzian spacetime, this becomes the physical four-volume.}
% & = \abs{\lambda} \abs{J} \, \dx^3 x_0 \, \dx t_0 \\
\dx \mathcal N & = \abs{\lambda} e^{3 Ht_0} \, \dx^3 x_0 \, \dx t_0
\end{align*}
where $(\vec x_0,t_0)$ are the coordinates at the time of nucleation.
\[ \ddx{\mathcal N}{V_{phys}} \approx \frac{\abs{\lambda}}{H^d} \frac{\dx R}{R^d} \]

% \[ \frac\Gamma{V_{\text{co}}} = \frac{9 H^4}{4\pi} \]

% \subsection{Approximations}

% { \centering
% % \begin{table}[h]
% \begin{tabular}{cccc}
% Geometry & Thin Wall & $R_0$ & $S_{\text{E}}$ \\
% Flat & Y & $\dfrac{N \sigma}{V(\phi_{\text{false}})-V(\phi_{\text{true}})}$ & $\dfrac{\sigma S_N(R_0)}{N+1}$ \\
% dS   & Y & $\dfrac{N \sigma}{e E_0}$ & $S$ \\
% Flat & N & $\dfrac{N \sigma}{e E_0}$ & $S$ \\
% dS   & N & $\dfrac{N \sigma}{e E_0}$ & $S$ \\
% \end{tabular}
% % \end{table} 
% \par}
