# Supplementary material for: How generic is eternal inflation?
Source: arXiv:2111.14218 source file (2021-12-26)
Supplement: Supplementary file 3 [file app_mc_methods.tex]

% \section{Master Flowchart}

% \begin{figure*}[p]
% \centering
% \includegraphics[width=14cm]{Figures/MasterFlowchart} % 10/18
% \caption{}
% \end{figure*}

\section{Measure C}

To determine if $\dot\phi$ comes in below the attractor bound, we integrate the coupled equations of motion for the homogeneous scalar field and the metric (only the scale factor $a$) backward in time, with initial conditions $\phi = \phi_{\text{sr}}$, $\dot\phi = \pm\sqrt{V(\phi_{\text{sr}})}$.
\begin{align} \ddot\phi &= -3 \frac{\dot a}{a} \dot\phi - V'(\phi) \\
\ddot a &= 8\pi G a \left( \dot\phi^2 - V(\phi) \right)
\end{align}
If the solution overshoots the peak rather than turning around, it would correspond to a velocity in the direction of $\phi_{\text{sr}}$ at some finite initial time.
If all forces were conservative we could assume that as we dial that initial velocity at the peak to zero, $\dot\phi$ approaches a value less than $\sqrt{V(\phi)}$ at $\phi_{\text{sr}}$.  The presence of Hubble friction complicates things somewhat, as it becomes possible that reducing this initial speed also reduces friction to the point that one gets greater $\dot\phi$ where slow roll begins.  
This can be tackled iteratively by overshoot-undershoot, trying to land with $\phi$ atop the peak at $t \to -\infty$.

\section{Instanton Pre-selection}

As illustrated in Figure \ref{fig:cdl_dominance},
the Hawking-Moss instanton dominates the transition between de Sitter minima if the top of the barrier is sufficiently flat \cite{A07transitionsbetween}:
\begin{equation} V(\phi) / m_{\text{Pl}}^2 \ll V''(\phi) \implies m_h \gg (8\pi)^{-1/2} \label{eq:cdl_cutoff} \end{equation}
This rules out the existence of CdL solutions; since the Hubble friction term in the Euclidean equation of motion has a wide valley floor of the inverted $V(\phi)$ over which to act, $\phi$ either cannot build up enough kinetic energy to reach the false vacuum or loses it to friction.
Well above the scale $m_h = (8\pi)^{-1/2}$, it is safe to assume that the transition is Hawking-Moss, and the rate is fast to compute.

\begin{figure}[ht]
\centering
\includegraphics[width=8.5cm]{Figures/scatter_024_2} % 9/29/2018
\caption{Fraction of models in which a Coleman-de Luccia instanton solution exists. At larger horizontal mass scales (flatter potential peaks), the Hawking-Moss instanton is dominant.}
\label{fig:cdl_dominance}
\end{figure}

At mass scales much smaller than \eqref{eq:cdl_cutoff}, we enter the thin wall regime, in which the CdL instanton dominates, and tends to terminate very near the true vacuum, traversing the barrier over a small interval in the Euclidean radial coordinate relative to $H_{\text{F}}^{-1}$.
In order to reduce program time allocated to computing transition rates in this regime, we first perform a check that inflation can start and end in the adjacent basin and that the maximum amount of inflation likely to occur is sufficient to produce $\mathcal N_e \gtrsim 55$.  
% In the absence of gravity, all instanton solutions terminate at the lower minimum; but accounting for the Hubble friction term allows the solution to terminate anywhere between the true vacuum and the top of the potential barrier.
% While $\phi$ could tunnel to a new value high on the opposite potential slope, the likelihood of landing above the ``edge'' of the barrier in the basin with a lower minimum, where $V(\phi_{\text{edge}}) = V(\phi_{\text{false}})$, and not saturating the limit of the Hawking-Moss instanton, is exceedingly low. 
%
Taking $\phi_{\text{edge}}$ such that \[V(\phi_{\text{edge}}) = 0.05\, V_{T} + 0.95\, V_{\text{bar}}\] as our trial starting point in the new basin, we search down the slope for the start (if slow roll conditions not already met at $\phi_{\text{edge}}$) and end of inflation.  
% (Since most successful diffusion events will be Hawking-Moss instantons, not much is at stake in the inconsistency of not requiring the slow roll conditions to be valid at the arrival point.)
If the slow roll conditions are valid all the way to the ``true'' vacuum, we conclude that inflation is eternal in the neighboring basin (barring consideration of any subsequent tunneling events).  Otherwise, we compute the number of $e$-folds that elapse between the start and end of inflation;
if it is greater than the 55 $e$-folds needed to obscure any potentially observable relics of the transition, then we proceed with the full instanton calculation to determine where precisely the field is deposited and at what rate.  

For intermediate mass scales, CdL instantons that terminate high on the barrier wall exist alongside thin wall and Hawking-Moss solutions, and we must integrate the bubble profile.

\section{Misc}

We sample multiple initial values from the same potential.
